# Supplementary material for: The Plot Thickens: Quantitative Part-by-Part Exploration of MLLM Visualization Literacy
Source: arXiv:2504.02217 source file (2025-04-03)
Supplement: Supplementary file 1 [file appendix.tex]

\begin{table}[h]
    \centering
    \begin{tabular}{lcc}
        \toprule
        \textbf{Dataset} & \textbf{Coef} & \textbf{$P>|t|$} \\
        \toprule
        const & -6.7024 & 0.000 \\
        referential\_title & -0.6076 & 0.013 \\
        dataset\_100\_stacked\_bar\_data.csv & 3.6710 & 0.000 \\
        dataset\_bar\_data.csv & -1.5086 & 0.004 \\
        dataset\_histogram\_data.csv & 3.8455 & 0.000 \\
        dataset\_line\_data.csv & 3.3633 & 0.000 \\
        dataset\_pie\_data.csv & 10.8077 & 0.000 \\
        dataset\_scatterplot\_data.csv & 4.0174 & 0.000 \\
        dataset\_stacked\_area\_data.csv & 2.5758 & 0.000 \\
        dataset\_stacked\_bar\_data.csv & -3.4474 & 0.000 \\
        plot\_type\_bar & -0.1064 & 0.897 \\
        plot\_type\_hist & 3.8455 & 0.000 \\
        plot\_type\_line & -0.0886 & 0.921 \\
        plot\_type\_scatter & -0.3186 & 0.699 \\
        plot\_type\_stacked\_bar & -0.1900 & 0.855 \\
        plot\_type\_stacked\_bar\_100 & -4.3050 & 0.000 \\
        color\_black & -0.4593 & 0.402 \\
        color\_burlywood & 0.2762 & 0.614 \\
        color\_chartreuse & 0.1308 & 0.811 \\
        color\_lightgray & -0.0349 & 0.949 \\
        color\_lightpink & -0.1163 & 0.832 \\
        color\_mediumvioletred & -0.0233 & 0.966 \\
        color\_red & 0.0203 & 0.970 \\
        color\_saddlebrown & 0.4215 & 0.442 \\
        color\_tomato & -0.0785 & 0.886 \\
        openai\_model & 2.5029 & 0.000 \\
        question\_type\_Determine Range & 16.8861 & 0.000 \\
        question\_type\_Find Anomalies & 10.1672 & 0.000 \\
        question\_type\_Find Clusters & 9.9422 & 0.000 \\
        question\_type\_Find Correlations/Trends & 18.3501 & 0.000 \\
        question\_type\_Find Extremum & 18.7489 & 0.000 \\
        question\_type\_Identify the Characteristic of Bins & 8.0500 & 0.000 \\
        question\_type\_Make Comparisons & 11.4372 & 0.000 \\
        question\_type\_Retrieve Value & 11.1889 & 0.000 \\
        \bottomrule
    \end{tabular}
    \caption{Regression Results}
    \label{tab:regression_results}
\end{table}
